# Supplementary material for: TRIAGE: Evaluating Prospective Metacognitive Control in LLMs under Resource Constraints
Source: arXiv:2605.13414 source file (2026-11-07)
Supplement: Supplementary file 1 [file appendix_documentation.tex]

% Dataset documentation appendix.
% Consider using structured templates such as:
%   - Datasheets for Datasets (Gebru et al.)
%   - Data Cards
%   - Croissant metadata description
%
% Include details on: motivation, composition, collection process,
% preprocessing, uses, distribution, and maintenance plan.
